# Supplementary material for: LeGO: Leveraging a Surface Deformation Network for Animatable Stylized Face Generation with One Example
Source: arXiv:2403.15227 source file (2024-03-22)
Supplement: Supplementary file 1 [file X_suppl.tex]

\clearpage
\setcounter{page}{1}

\maketitlesupplementary

\section*{Overview}
\label{sec:Overview}
In this supplementary material, we present implementation details in Section~\hyperref[sec:A]{A}. Section~\hyperref[sec:B]{B} contains the details of the LeGO architecture. Section~\hyperref[sec:C]{C} covers additional experiments and their corresponding details. Section~\hyperref[sec:D]{D} is dedicated to visualizing example  results of the applications of our method. Lastly, Section~\hyperref[sec:E]{E} presents additional results. For additional results, please visit the project page~\href{https://kwanyun.github.io/lego/}{https://kwanyun.github.io/lego/}.

\section*{A. Implementation Details}
\label{sec:A}
The implementation of LeGO including the surface deformation
networks $D_S$ and $D_T$, and MAGE on an Nvidia RTX 3090 GPU. The implementation details are sequentially presented, in the order of  with $D_S$, $D_T$, MAGE, and the baselines for the experiments in the following paragraphs.

\paragraph{Training $D_S$} To deform a template face to a person with a different identity and expression, we trained the source surface deformation network $D_S$ using the FLAME~\cite{li2017learning} parameter $\Phi$ and its corresponding face mesh, as described in the main paper. We sampled 100k instances of $\Phi$ and their corresponding faces for self-supervised training, with $\Phi$ being sampled from a uniform distribution to learn diverse identities and expressions. We jointly trained $\mathcal{M}_{shape}$, $\mathcal{M}_{exp}$, and $D_S$ for 400 epochs with a fixed learning rate of 1e-6. We adopted the SIMS approach to enable $D_S$ to handle diverse topologies by training it using surface points instead of only sampling from mesh vertices.

\begin{figure}[h]
\centering
\includegraphics[width=\linewidth]{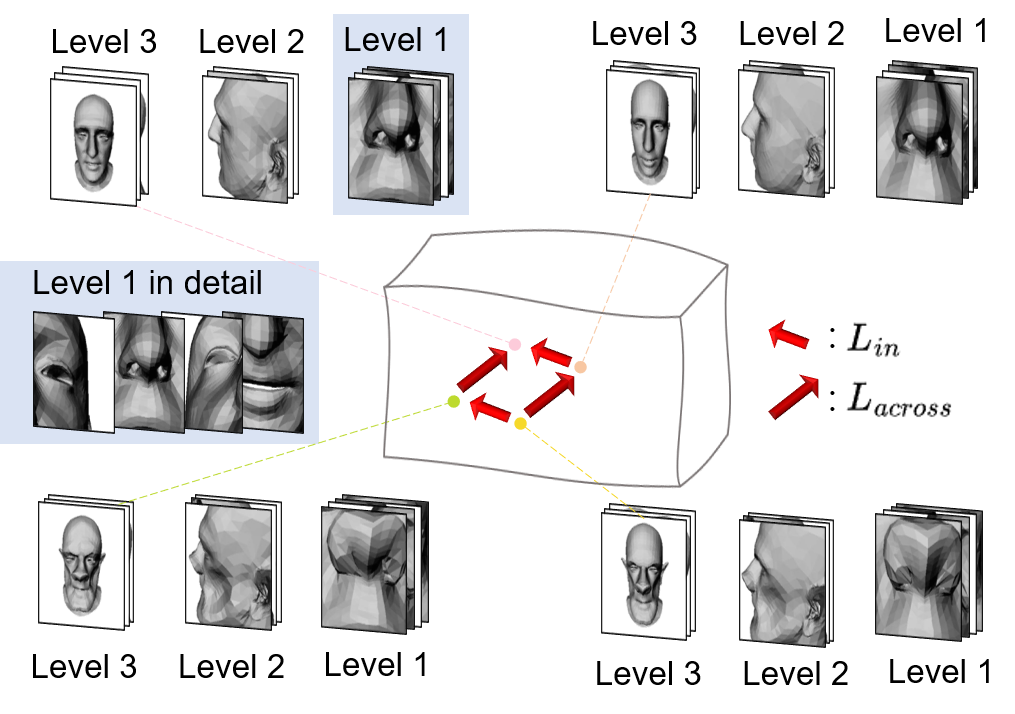}
\caption{Detailed illustration of $L_{in}$ and $L_{across}$ with hierarchical rendering. The blue box shows an example of the predefined pivots of hierarchical rendering.}
\vspace{-2pt}
\label{fig:mtg}
\end{figure}

\paragraph{Training $D_T$} To modify the template face to incorporate styles while maintaining the same identity and expression as $D_S$, we trained the target surface deformation network $D_T$ following the procedure outlined in the main paper. The training began with an initial learning rate of 3e-5, which gradually decreased to 1e-5 over 2,000 iterations. The balancing weights in Equation (9) in the main paper, $\lambda_{\text{vert}}$,$\lambda_{\mathrm{CLIP}}$, $\lambda_{\text{in}}$, $\lambda_{\text{across}}$, and $\lambda_{\text{style}}$ were fixed at 80, 2e-3, 6e-3, 6e-3, and 4e-3, respectively. 

During the training of $D_T$,  we adopted a hierarchical rendering approach comprising three levels. The first level, featuring the most enlarged views, focused on rendering local facial parts such as the eyes, nose, and lips (illustrated in the blue box in Figure~\ref{fig:mtg}). The second level includes close-up views of faces from three directions, encompassing the front and sides of the face. The last level comprises full-face views from the same directions.

\paragraph{Training MAGE} MAGE functions as an encoder that transforms faces with diverse topologies into the latent space of LeGO, specifically into the shared latent space of $D_S$ and $D_T$. NFR~\cite{qin2023neural} encoders were fixed during training, while ID2ID, exp2exp, and latent mapper were jointly trained. The model was trained with an initial learning rate of 3e-4, which gradually decreased to 5e-5 over 12,000 iterations.

\begin{figure}[h]
\centering
\includegraphics[width=\linewidth]{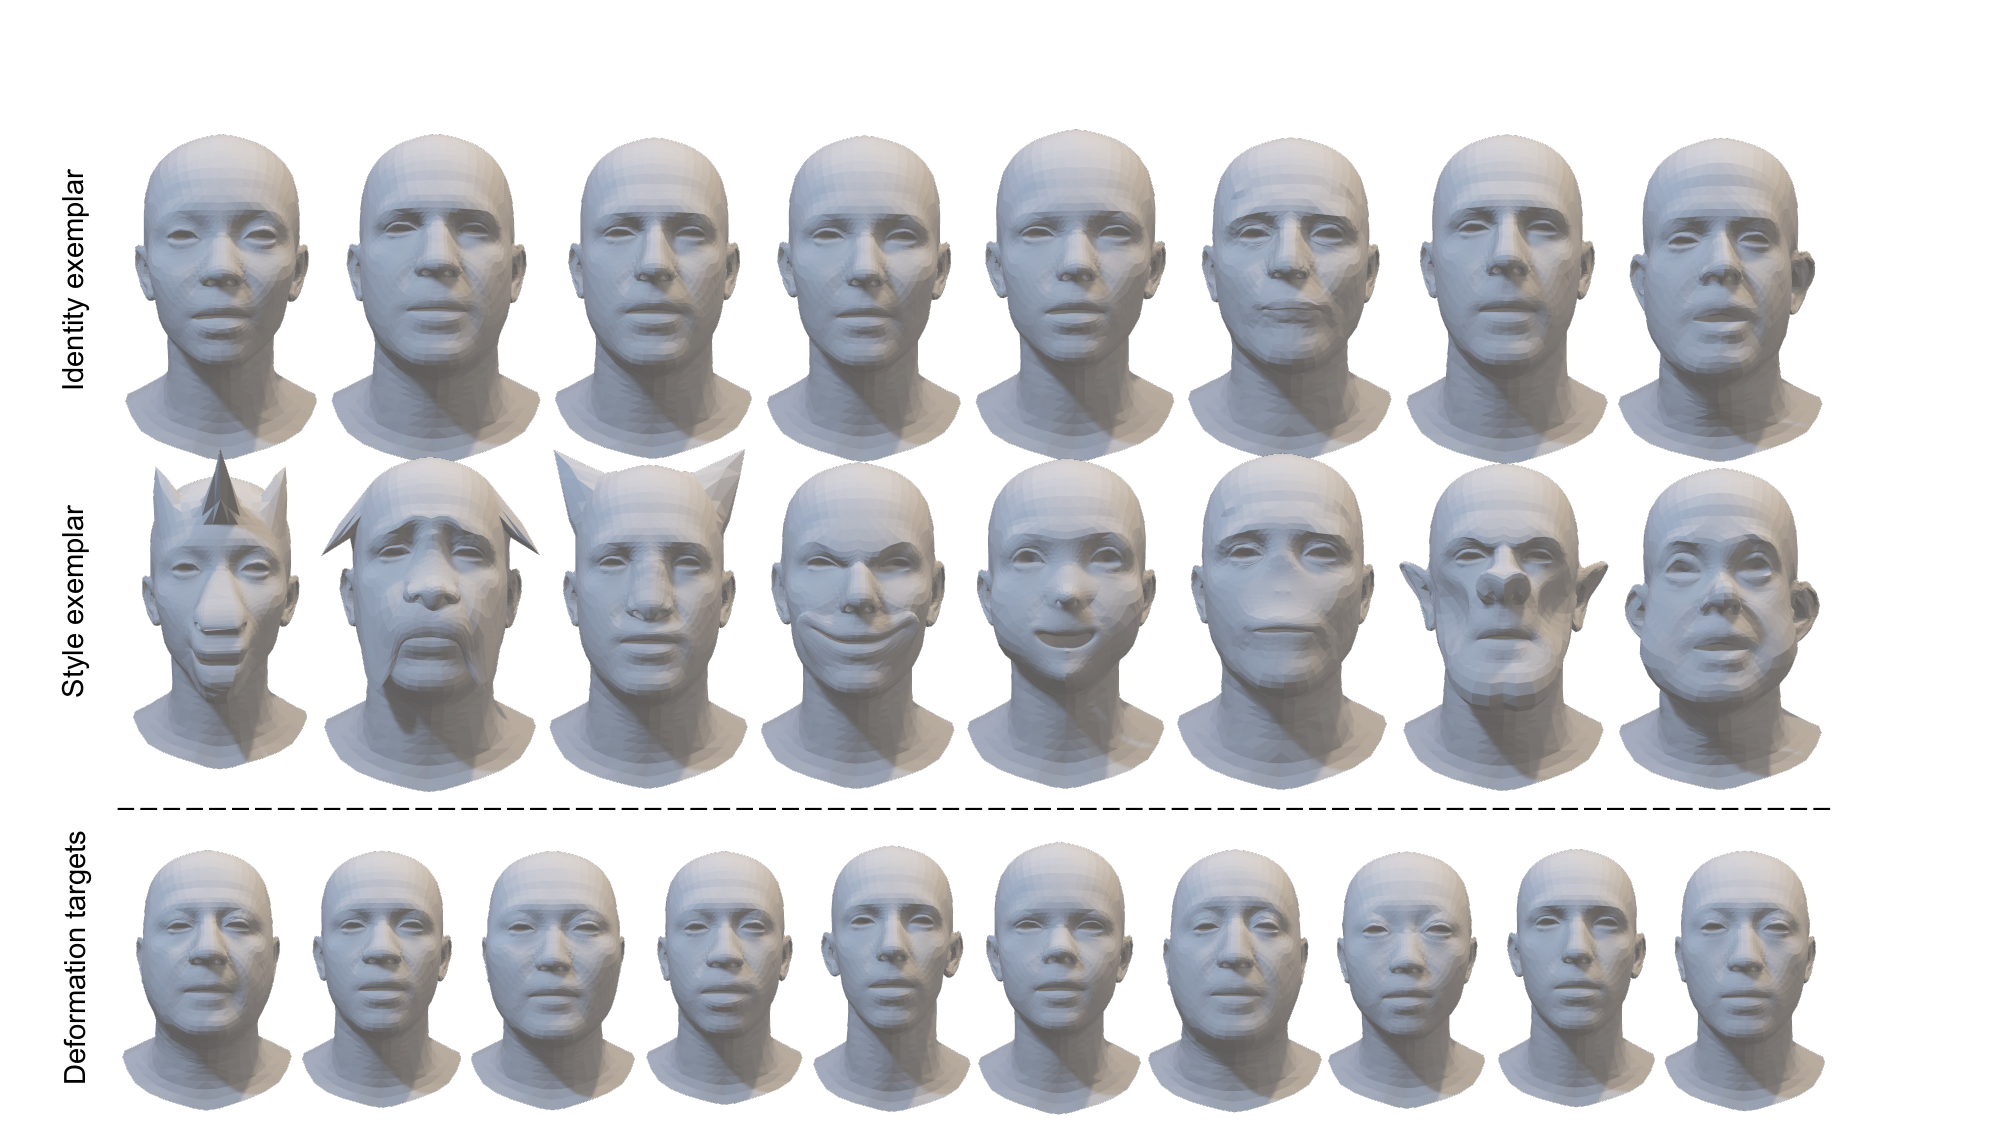}
\caption{First two rows are identity exemplar mesh and style exemplar mesh in our dataset, created for fine-tuning. Last row shows deformation target meshes for experiments}
\vspace{-4pt}
\label{fig:dataset}
\end{figure}
\begin{figure*}[t]
\centering
\includegraphics[width=0.95\linewidth]{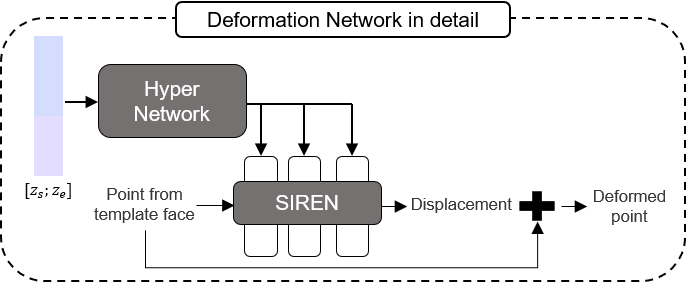}
\caption{Visualization of deformation network in detail.}
\label{fig:deformationnet}
\end{figure*}

\paragraph{Baseline Methods} All baseline methods were using their default settings as specified in their respective papers or the official code provided by the authors. 
As specified in the main paper, we utilized 8 different faces with corresponding manually crafted meshes as a dataset, which are shown in Figure~\ref{fig:dataset}. We also randomly sampled another 10 different identities without expressions from FLAME decoder as deformation targets for experiments.
For the text-based methods~\cite{gao2023textdeformer,ma2023x}, we used the deformation target as the source template mesh and text to specify the target style. Eight text prompts that describe styles are as follows: "Bulldog makeup", "Disney Dwarf", "Exaggerated smile", "Musical Cats", "Orc", "Person with unicorn horn", "Person without nose", and "Pixar child".
\vspace{4mm}

\section*{B. LeGO Architecture}
\label{sec:B}

\subsection*{B.1 Deformation Network Architecure}
The architectures of $D_S$ and $D_T$ are designed to compute the displacement of a point, either from a vertex or surface, and produce a deformed face output. The architectures are inspired by DD3C~\cite{jung2022deep}.
The architecture of the deformation network is illustrated in Figure~\ref{fig:deformationnet}. The latent code [$z_s$;$z_e$] enters the hypernetwork, modifying the parameters of the SIREN MLP~\cite{sitzmann2020implicit}. Subsequently, as the point from the template face traverses the network, the displacement is added to the point, determining the output position.
\vspace{2mm}
\subsection*{B.2 Rationale Behind Using the Deformation Network}
%A basic question might arise: why do we train a deformation network instead of simply adding the displacement? The easiest answer is that it cannot handle the diverse input and output. However, upon closer inspection, another issue arises: naively transferring displacement from one face to another can lead to severe artifacts, especially when the identities of the source face from the example pair and the target face are significantly different
The main reason to utilize a deformation network instead of simply adding an displacement lies in the inability of handling diverse inputs and outputs when the simple method is used. Another reason is to avoid severe artifacts that may occur when the identity of the deformation target and identity exemplar mesh are too different to directly transfer the displacement from one face to another. Examples of these artifacts are illustrated in Figure~\ref{fig:naiive}.

\begin{figure}[h]
\centering
\includegraphics[width=1.05\linewidth]{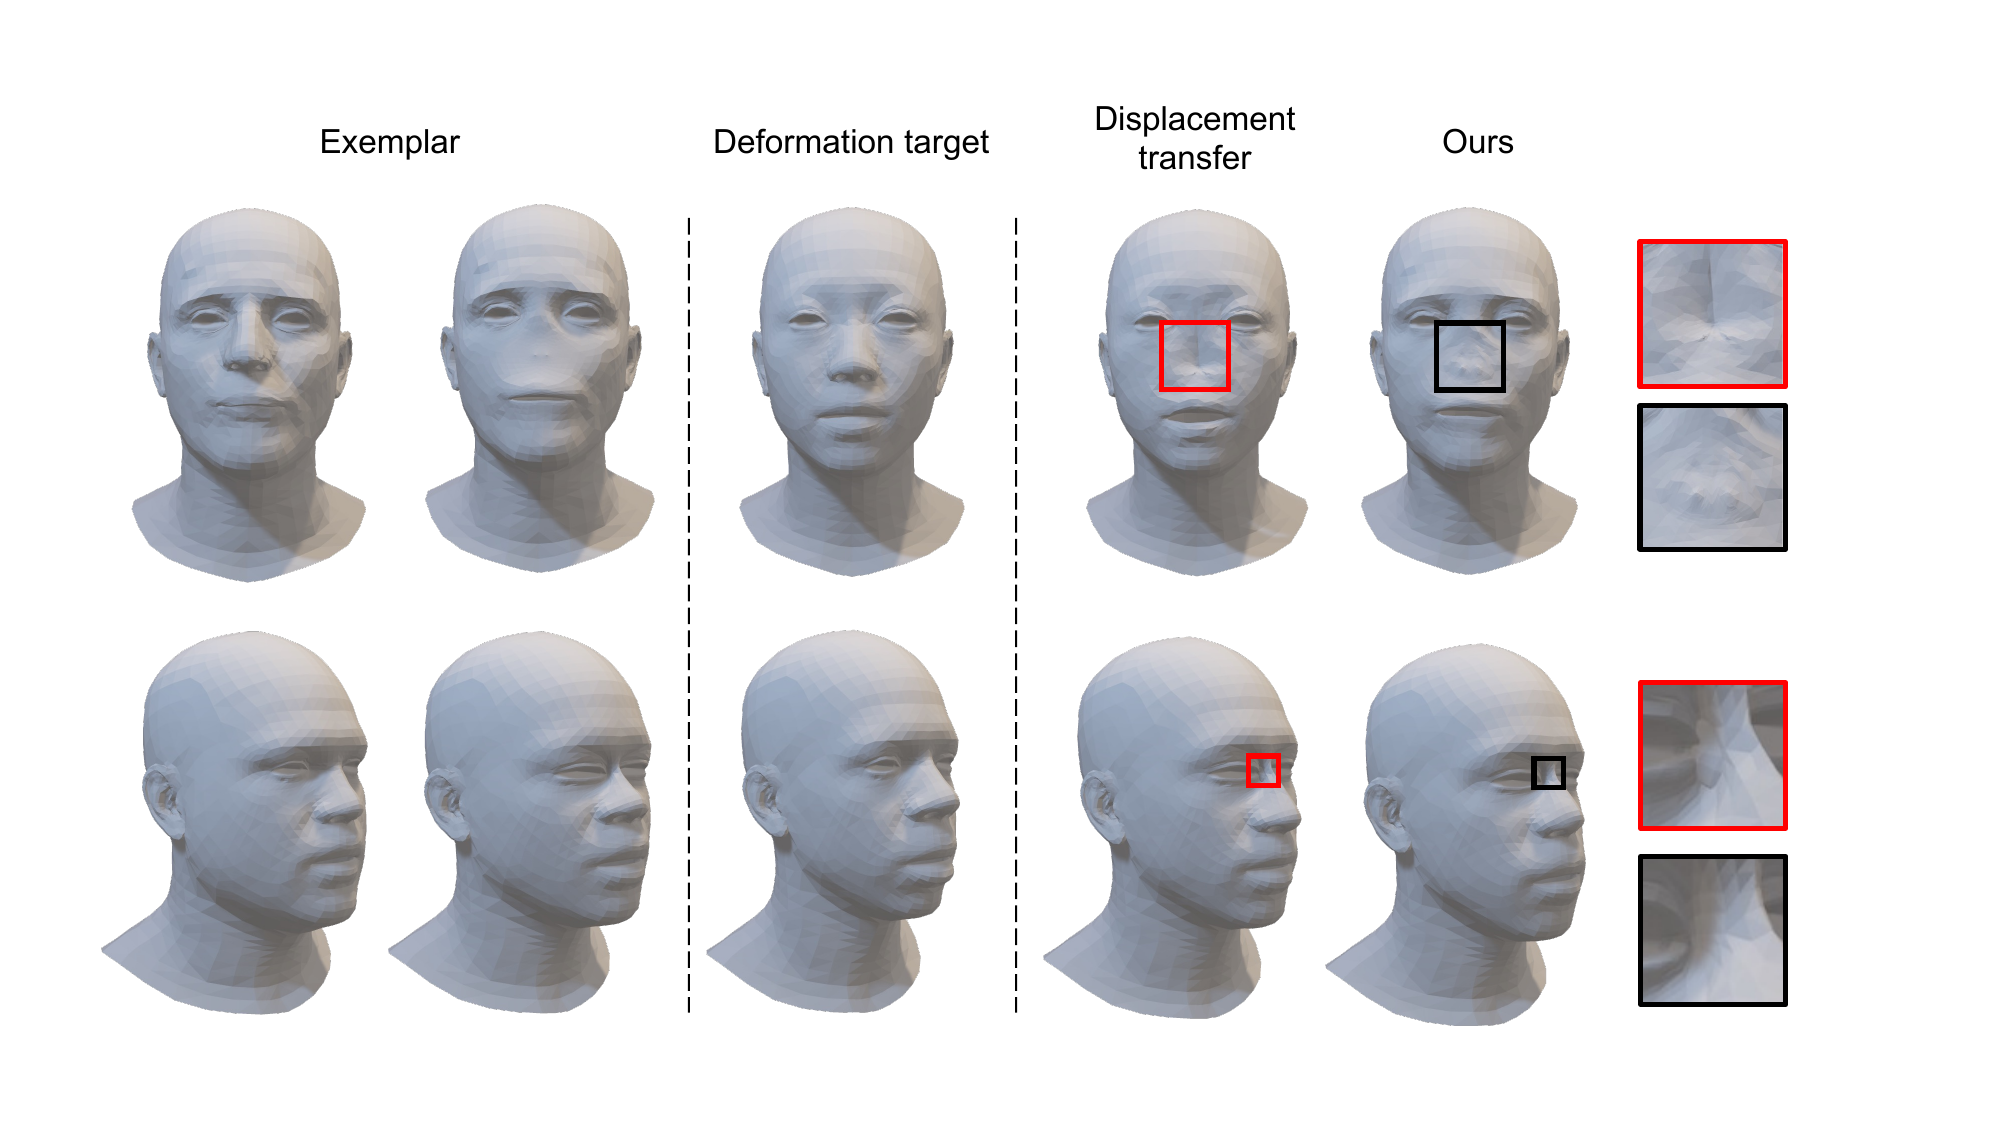}
\caption{Artifacts occurred by simple displacement transfer. The red boxes show the close-up views. The boxes colored in red show the result of simple dispacement with artifacts(sunk nose and penetration on eye region) unlike Ours, colored in black.}
\label{fig:naiive}
\end{figure}

\begin{figure*}[h]
\centering
\includegraphics[width=\linewidth]{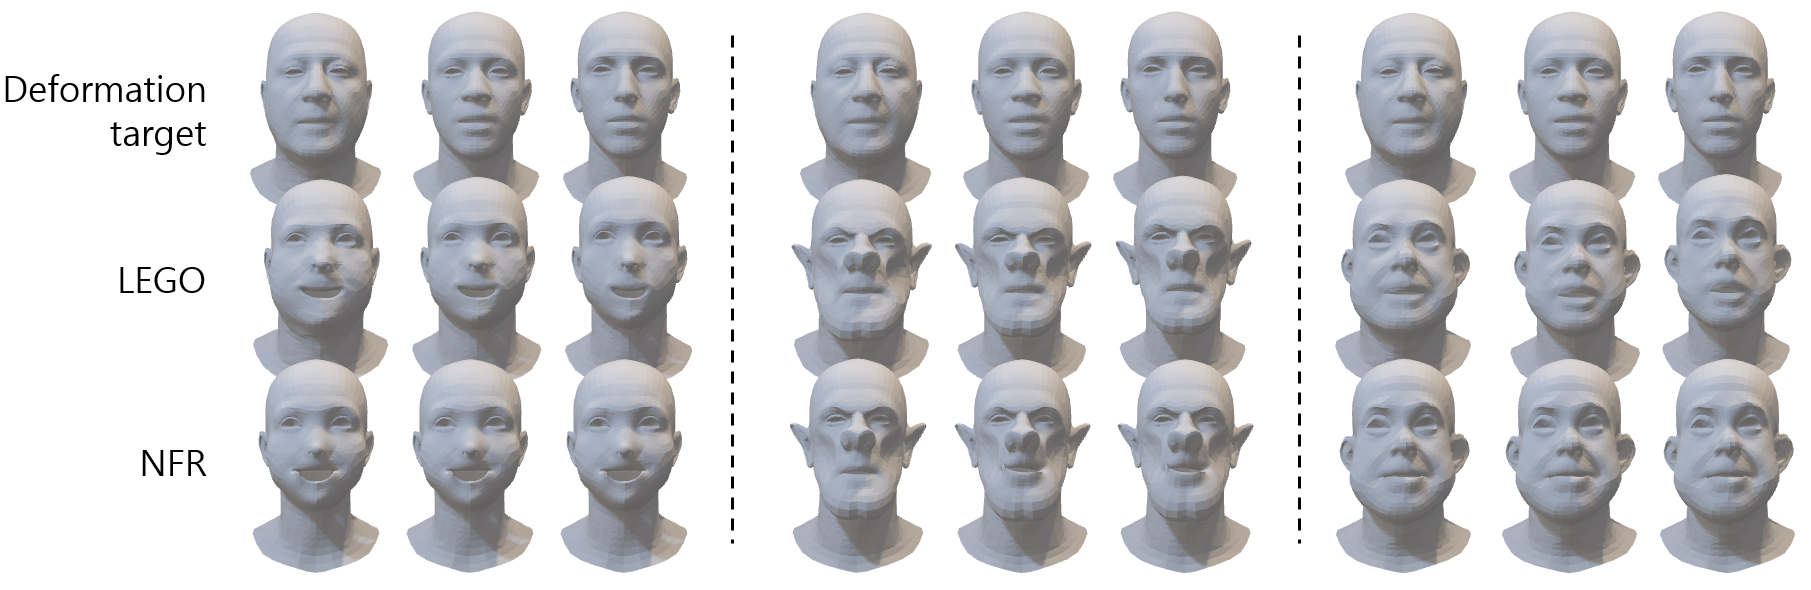}
\caption{Comparison with NFR and LEGO. Becaus NFR is designed for expression transfer, it's expression encoder cannot preserve identity.}
\label{fig:nfr}
\end{figure*}
\section*{C. Additional Experiments}
\label{sec:C}
\subsection*{C.1 Comparison with NFR}
\revised{NFR~\cite{qin2023neural} is a method that can transfer the expression of a target facial mesh to an unrigged identity mesh of arbitrary topology. Because NFR is specifically designed for expression transfer, it is difficult for the method to preserve both identity and style in the resulting mesh. However, because NFR is the backbone of MAGE, we compared it with our method. As shown in Figure~\ref{fig:nfr}, although NFR could generate a stylized mesh, it failed to preserve the original identity, resulting in all similar outcomes that reflect the style exemplar.}

\subsection*{C.2 Ablation on Direct Style Loss}
As stated in the main paper, "Ours" and "Ours w. direct $L_{style}$" loss produced the least amount of surface artifacts. Here, the style loss that directly compared $D_T([{z_s}^{samp};{z_e}^{samp}])$ and $M_T$, it forced the stylized face to have the same expression as $M_T$. In contrast, ours that compared $D_T([{z_s}^{samp};{z_e}^{ref}])$ and $M_T$ successfully maintained animatability. This is illustrated in Figure~\ref{fig:animation}.
\begin{figure*}[h]
\centering
\includegraphics[width=\linewidth]{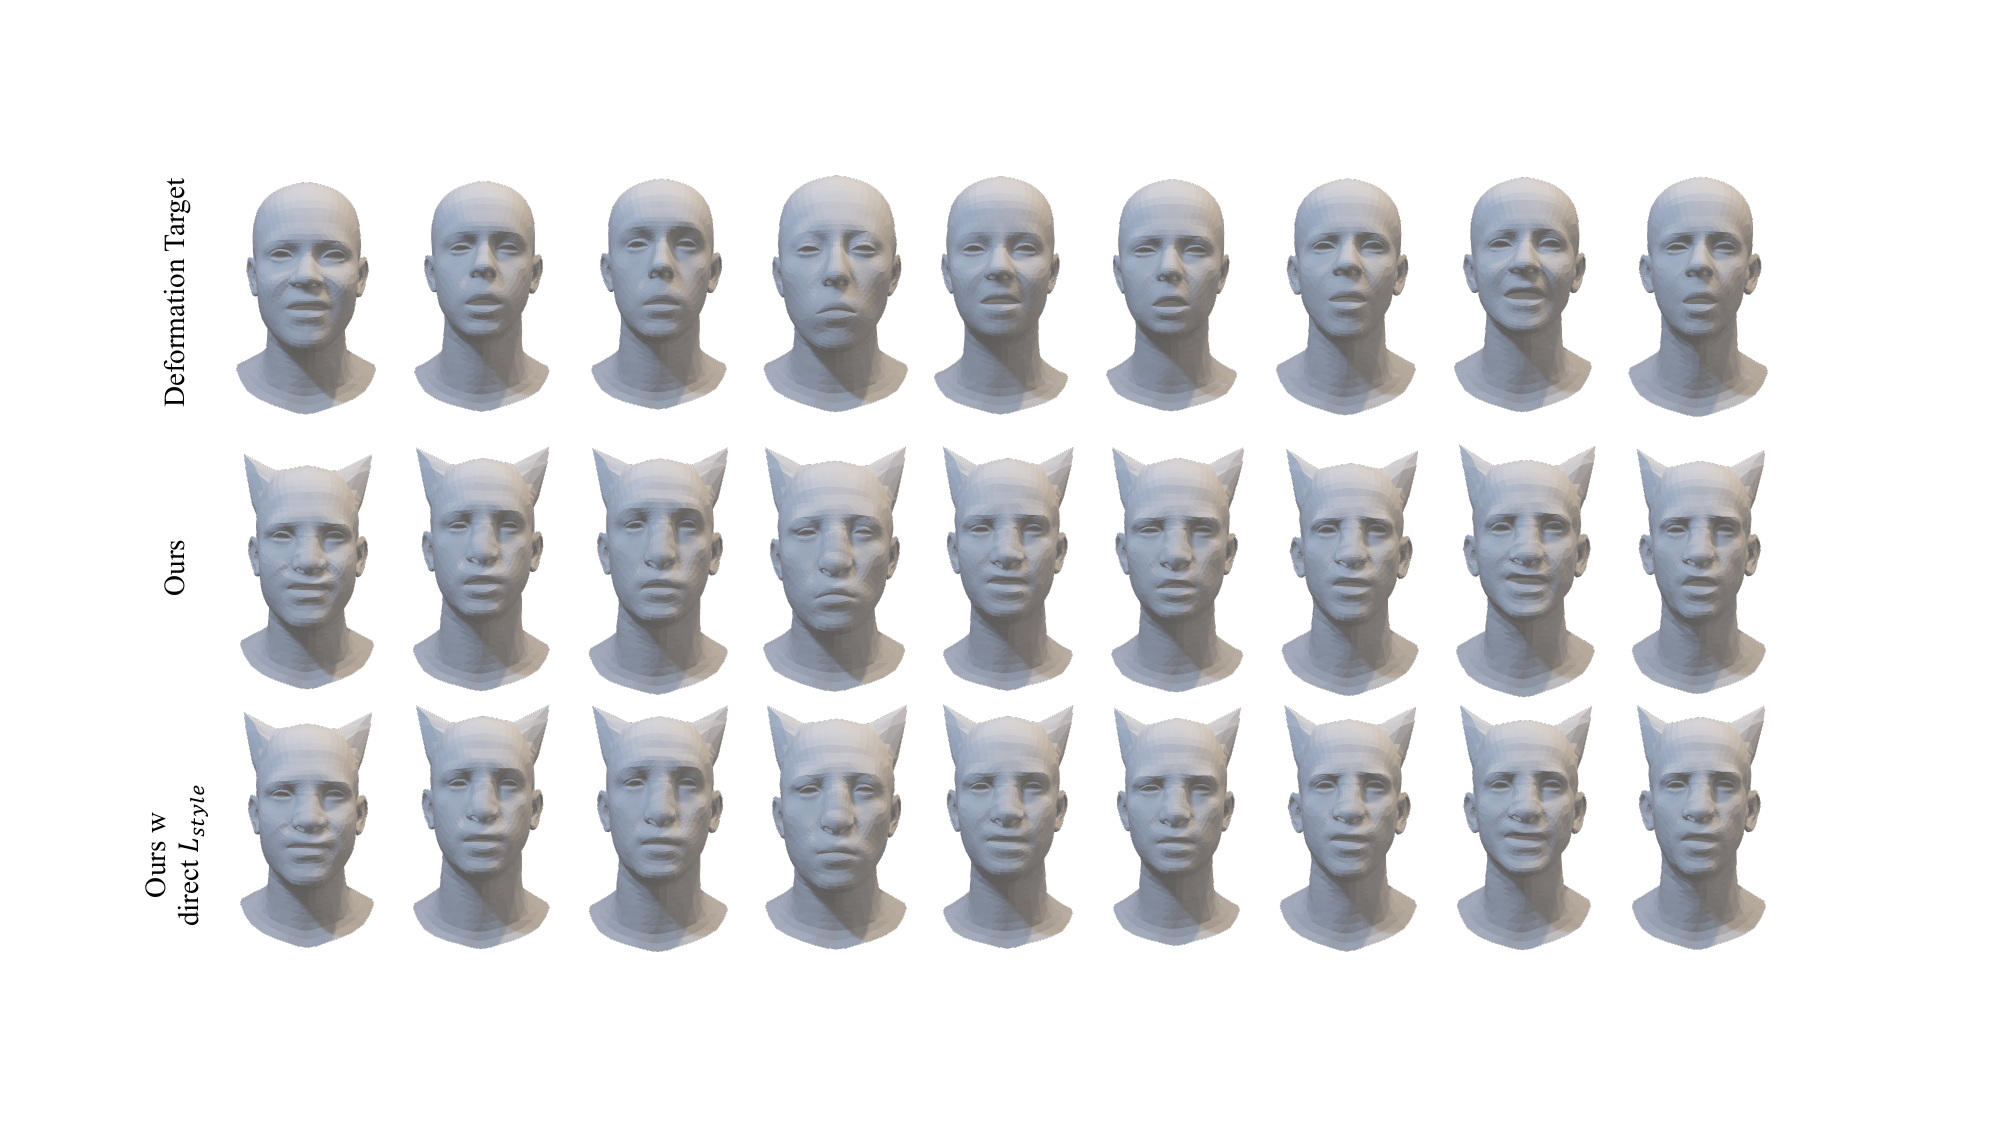}
\caption{Comparison with Ours and Ours w. direct $L_{style}$. Both methods generated the style well while Ours followed the expression from the deformation target better compared to Ours w. direct $L_{style}$.}
\vspace{-4pt}
\label{fig:animation}
\end{figure*}

\begin{figure}[h]
\centering
\vspace{-4pt}
\includegraphics[width=\linewidth]{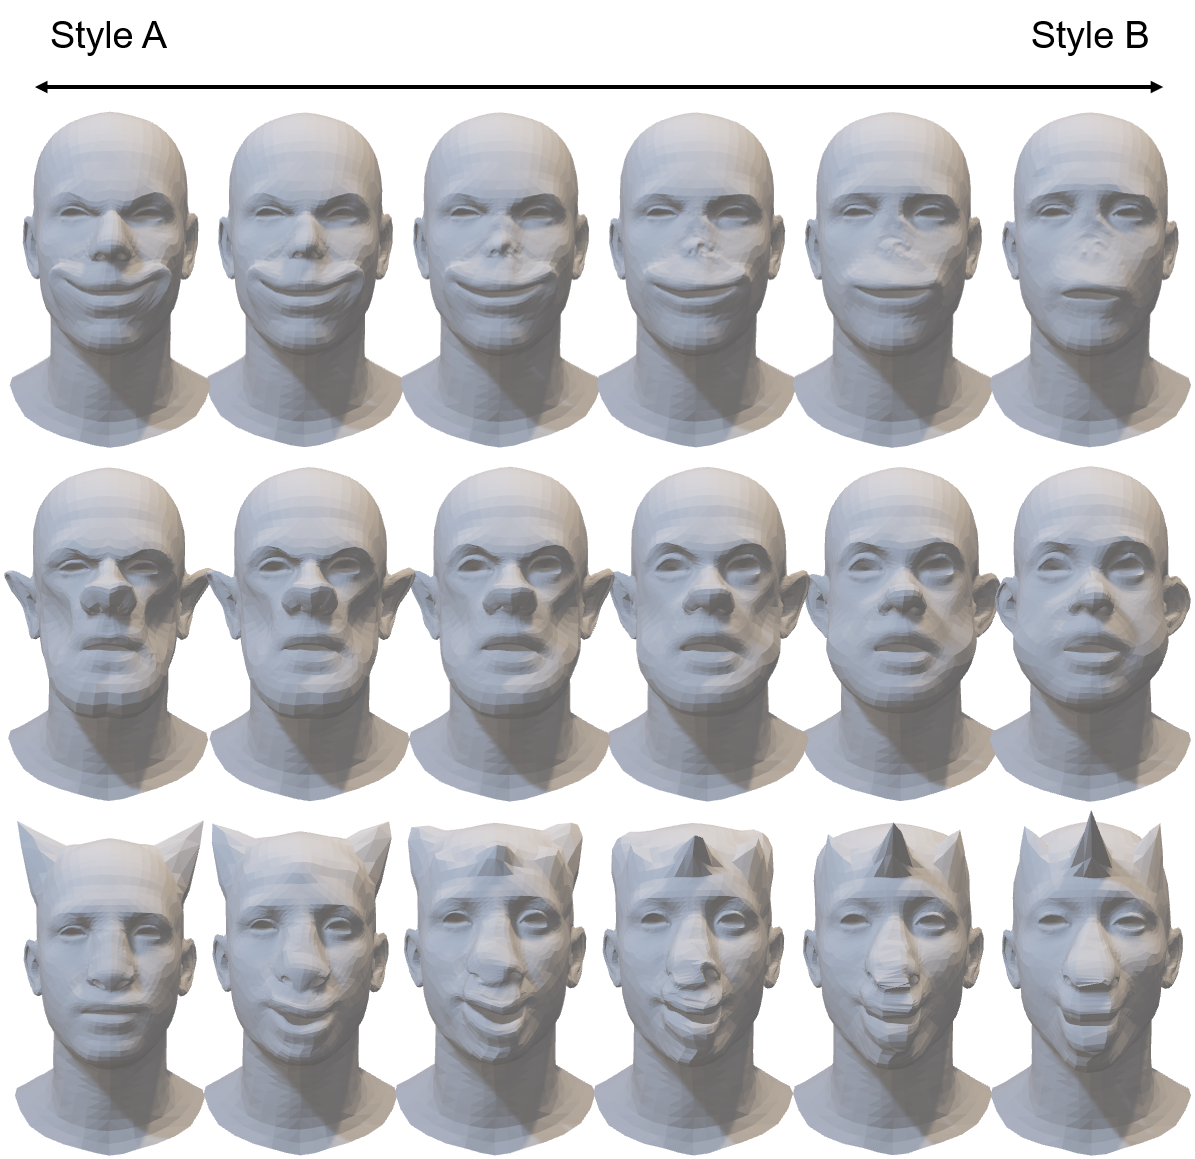}
\caption{Additional results of style interpolation.}
\vspace{-6pt}
\label{fig:interpolation}
\end{figure}

\section*{D. Applications}
\label{sec:D}

\subsection*{D.1 Visualization of Results Produced by the Applications.}
We present additional results of style interpolation in Figure~\ref{fig:interpolation}. These results demonstrate that our method can effectively construct the latent space for identities and styles, ensuring that even when mixing weights, the person's identity remains unchanged while the styles transition smoothly. This finding inspired the generation of new styles by blending existing ones. Additionally, we showcase further results on generating stylized 3D faces from 2D portraits, indicating that our method does not require a mesh as input; instead, any image can be used to create a stylized face with a specific identity, thereby broadening the practical application of our method.

\begin{figure*}[h]
\centering
\includegraphics[width=0.75\linewidth]{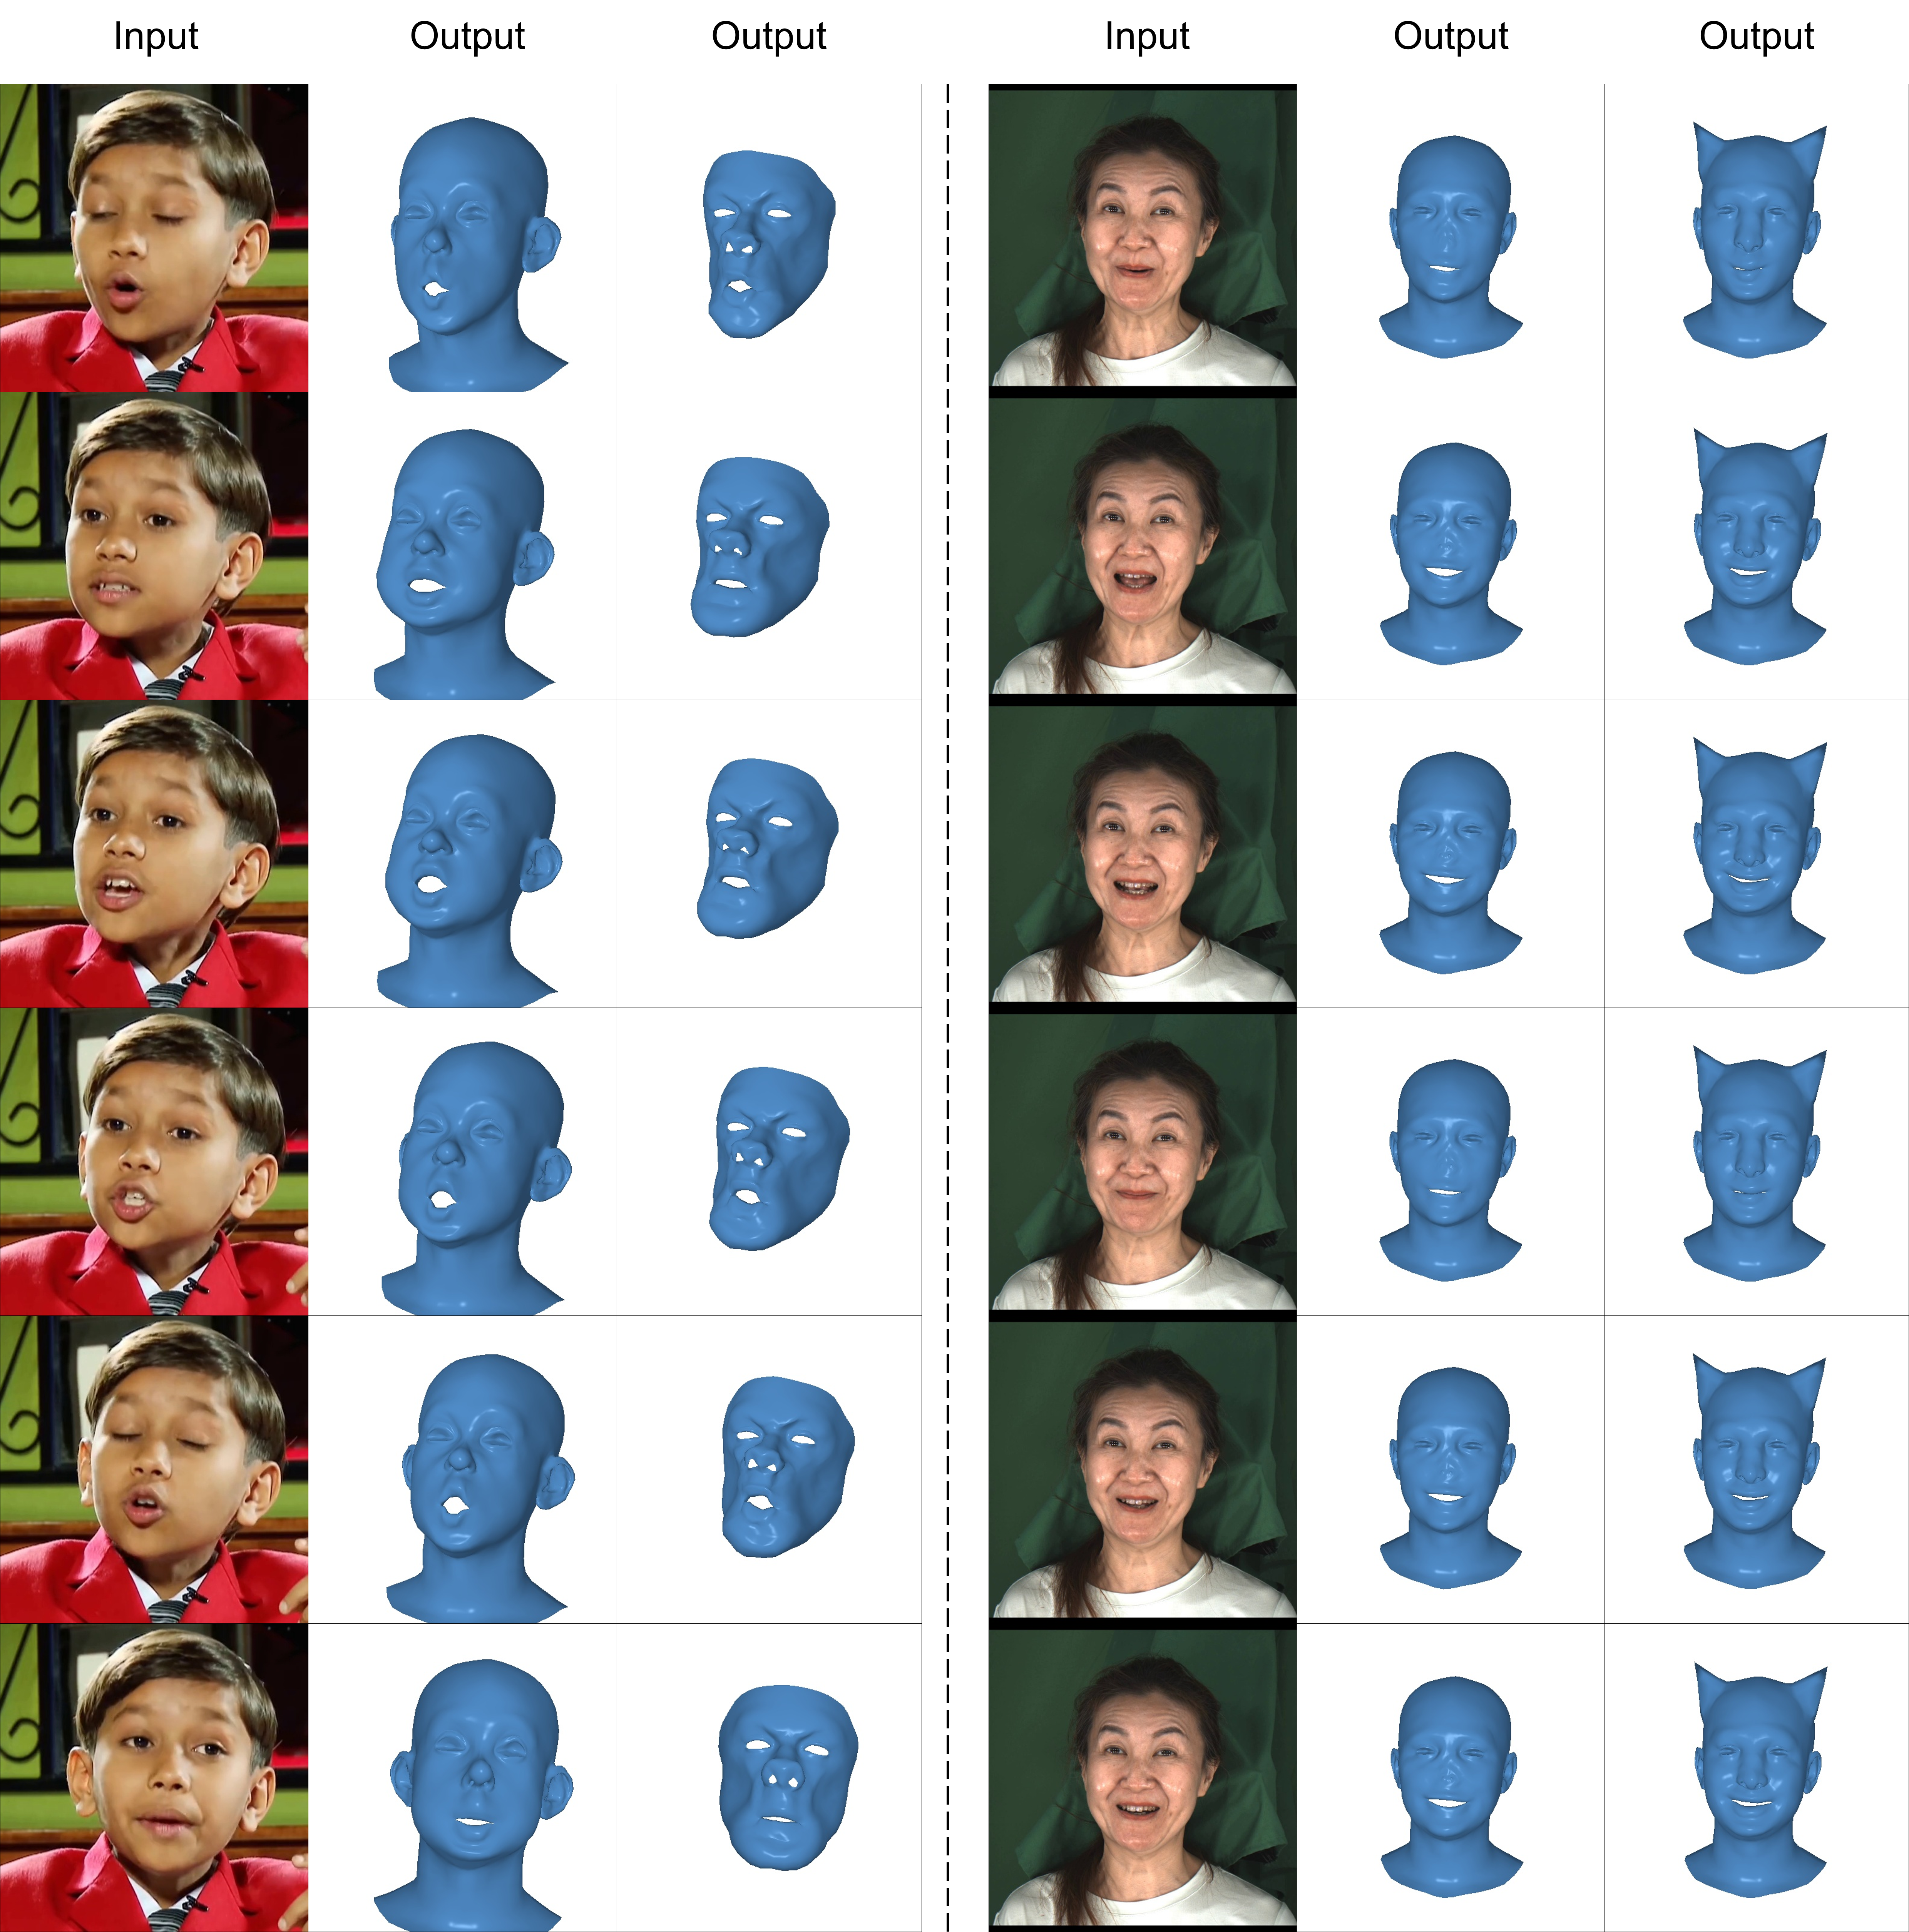}
\vspace{-8pt}
\caption{Retargeting from video, two different styles are shown for each input. Left examples are from Talking-head-1KH~\cite{wang2021facevid2vid} and right examples are from MEAD dataset~\cite{wang2020mead}.}
\vspace{-10pt}
\label{fig:video}
\end{figure*}

\subsection*{D.2 Retargeting from Video}
Retargeting is one of widely used applications in animation in which target follows the animation of the source. We performed an additional experiment on video driven stylized 3D face retargeting. Using a metrical photometric tracker~\cite{zielonka2022towards}, we can obtain the shape and expression parameters of FLAME from video, which can be directly adopted to LeGO. From these parameters, we achieved 3D stylized face retargeting as shown in Figure~\ref{fig:video}. Additional results are shown in the supplementary video.

\section*{E. Additional Results}
\label{sec:E}
We present additional stylization results produced by LeGO trained with a paired exemplar. Figures~\ref{fig:add1}, ~\ref{fig:add2} and ~\ref{fig:add3} display the results of all eight styles and deformation targets with different topologies.

\begin{figure*}[h]
\centering
\includegraphics[width=0.88\linewidth]{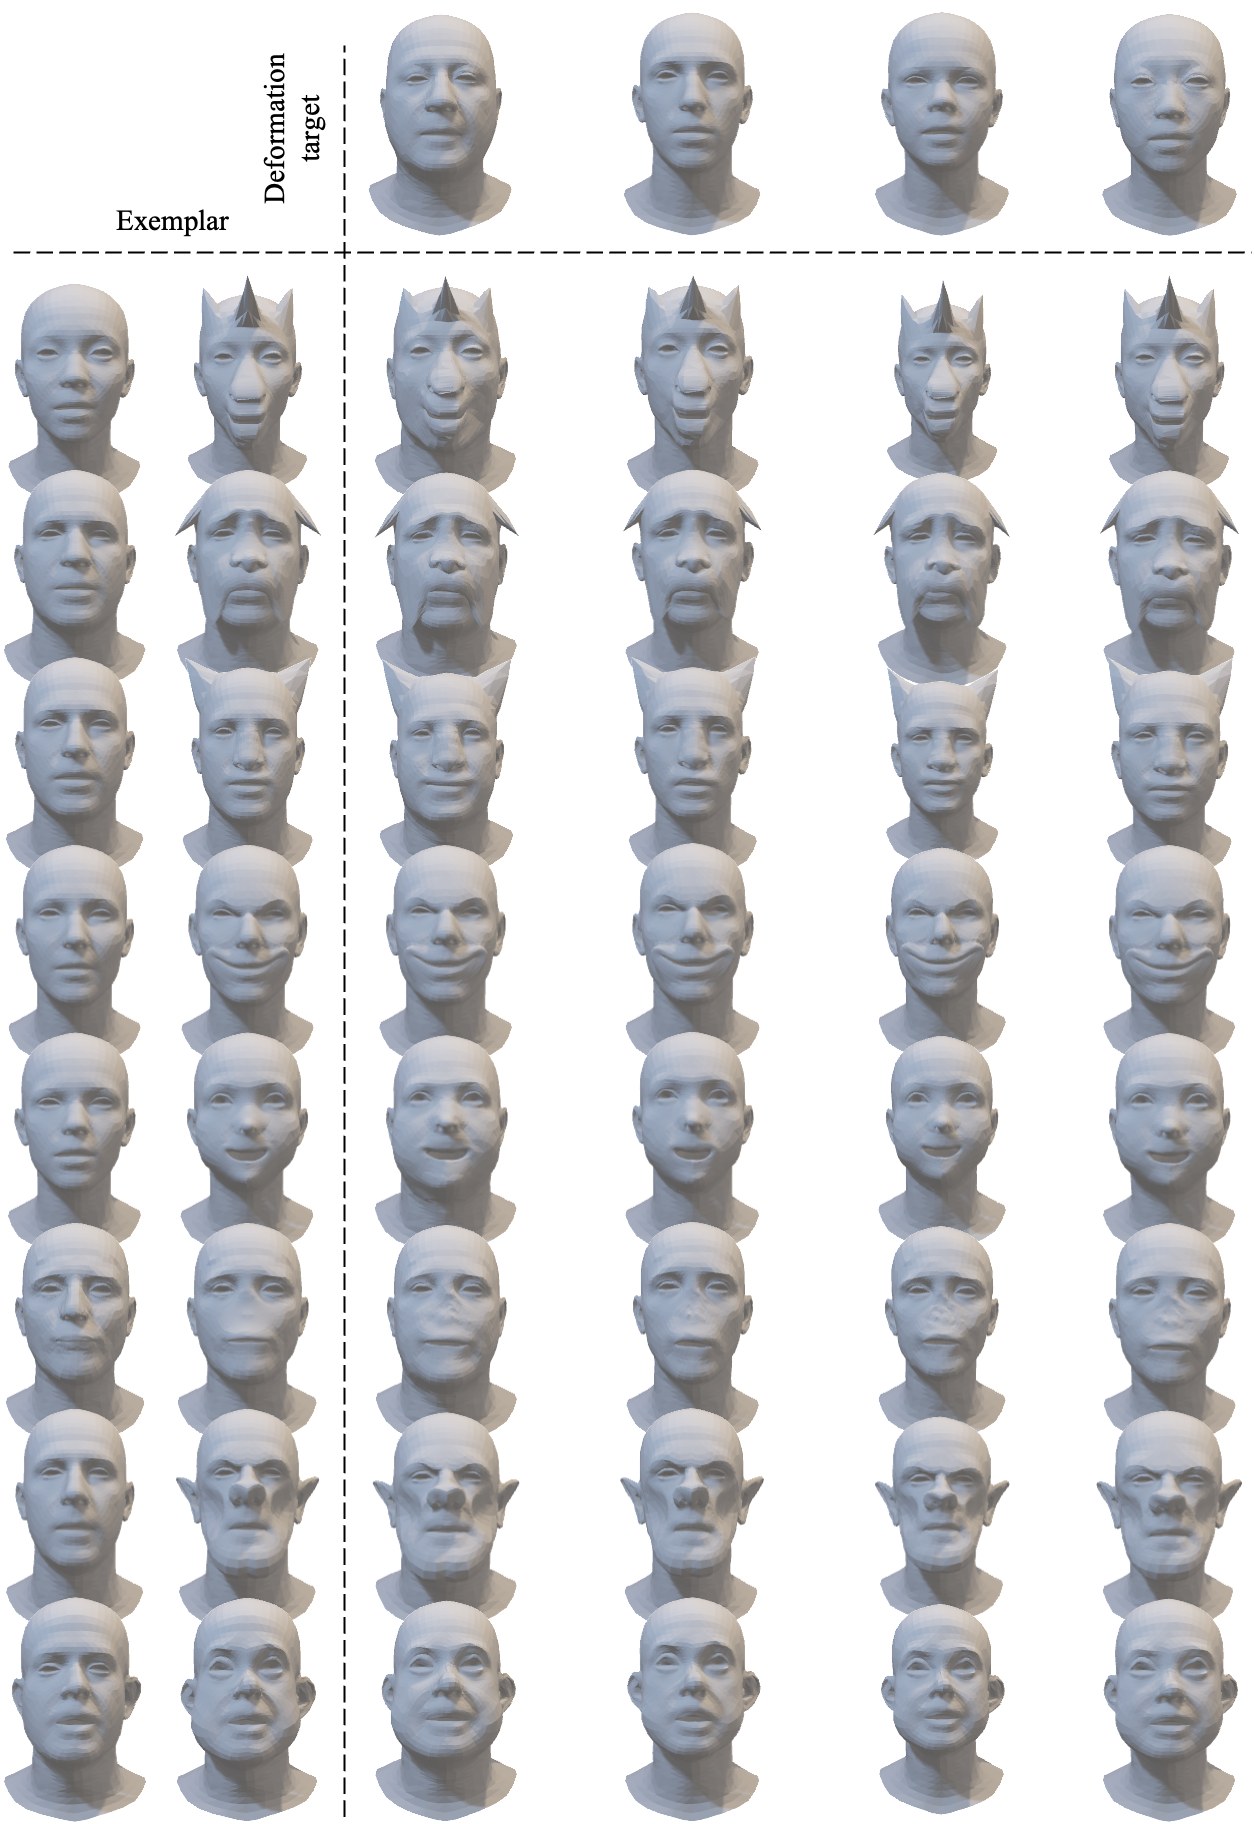}
\caption{Additional results on all 8 different styles.}
\vspace{-5pt}
\label{fig:add1}
\end{figure*}
\begin{figure*}[h]
\centering
\includegraphics[width=0.88\linewidth]{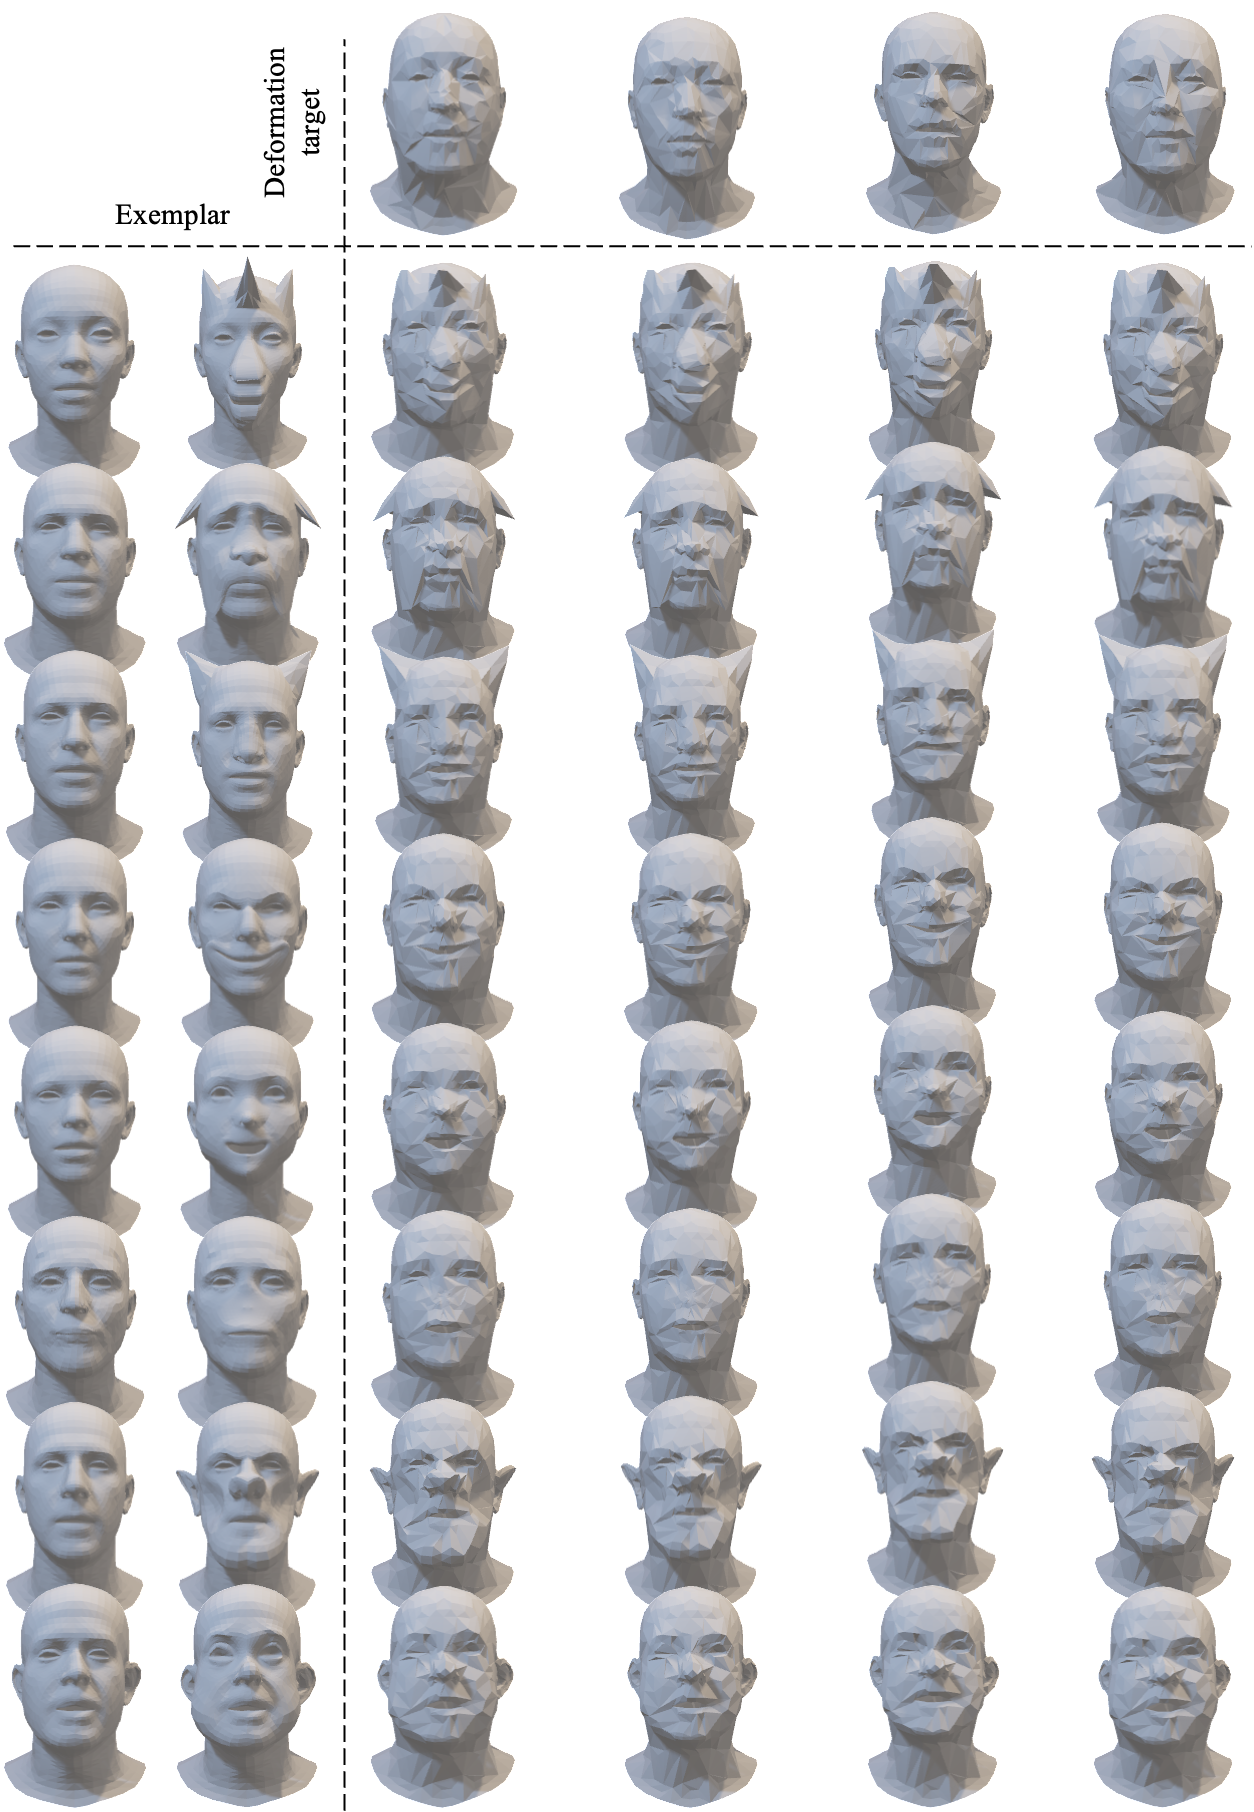}
\caption{Additional results on all 8 different styles.}
\vspace{-5pt}
\label{fig:add2}
\end{figure*}
\begin{figure*}[h]
\centering
\includegraphics[width=0.88\linewidth]{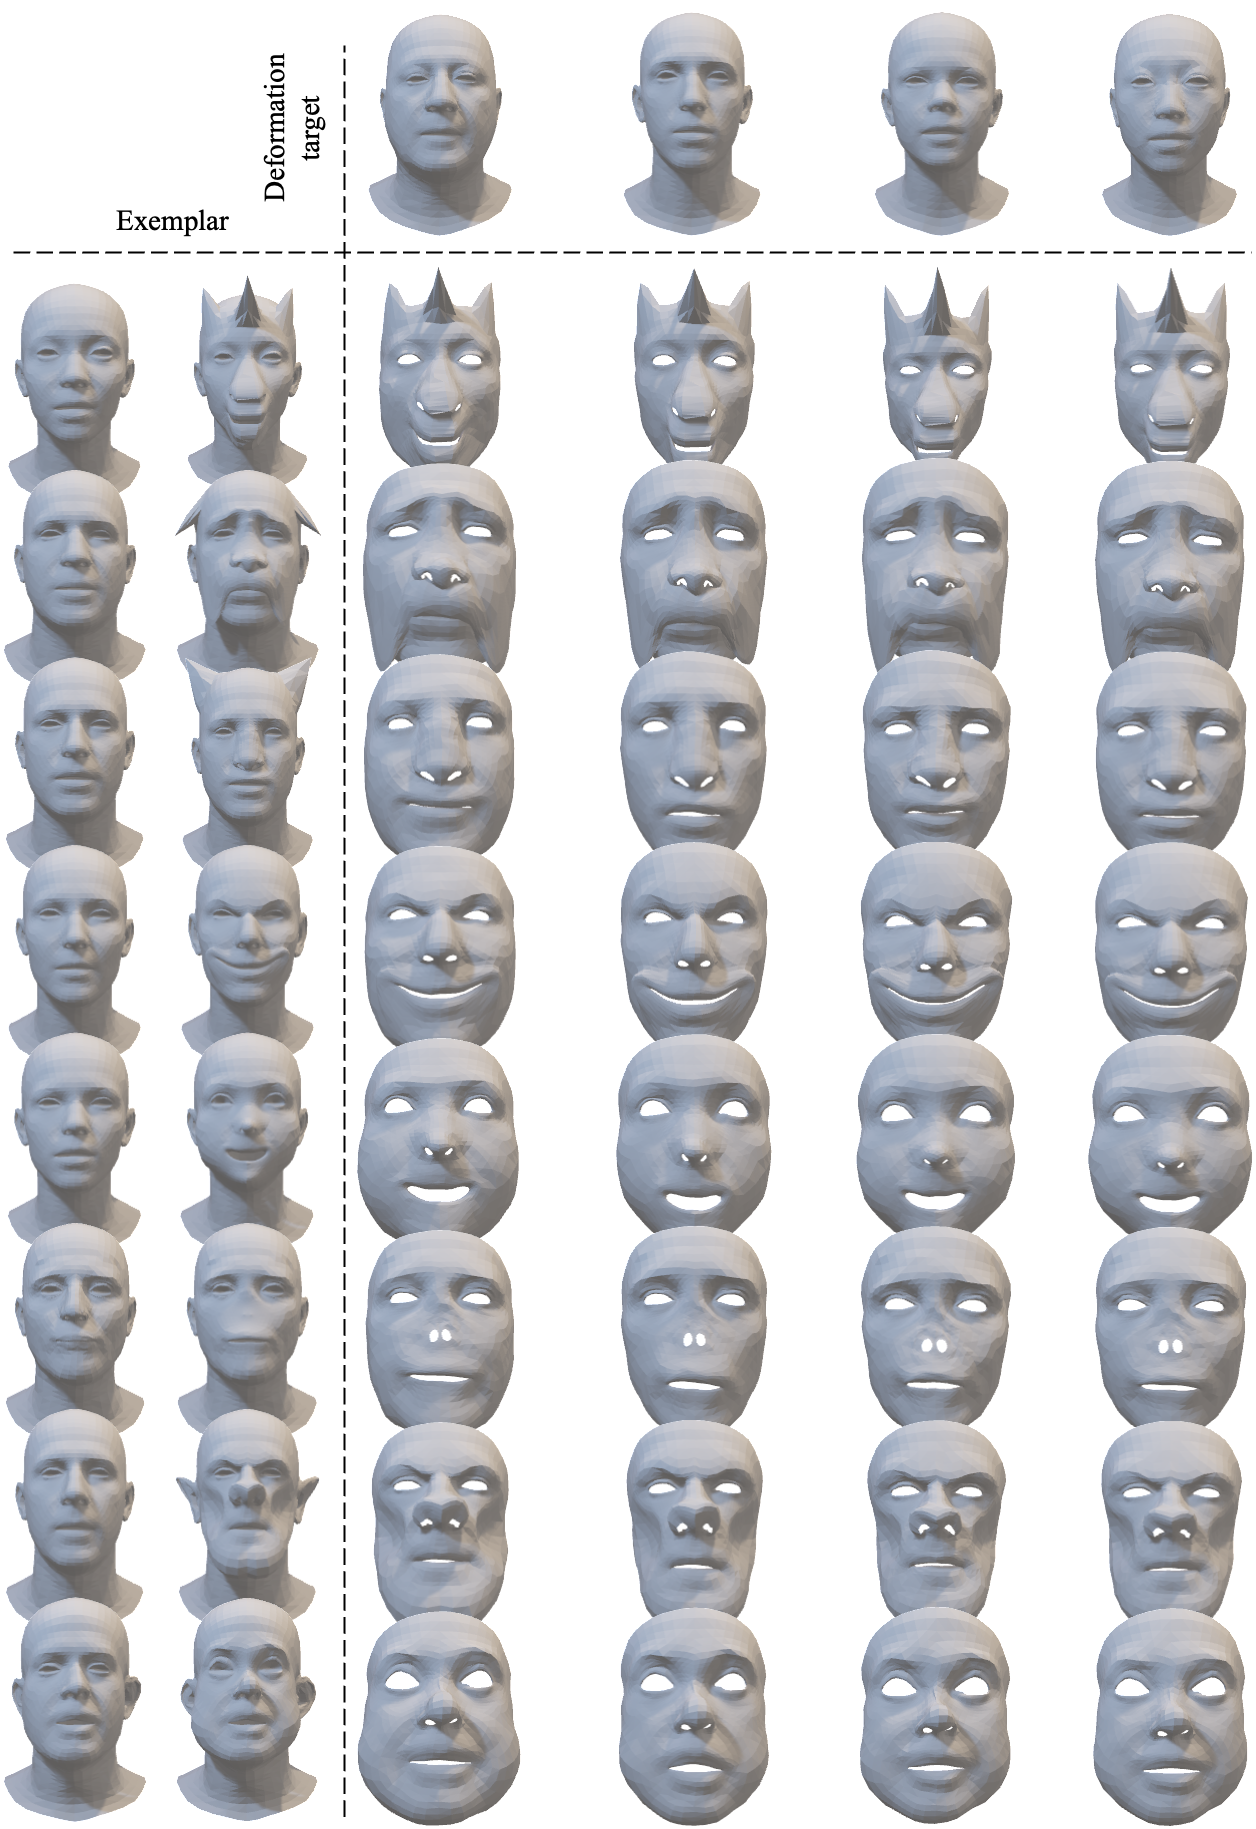}
\caption{Additional results on all 8 different styles.}
\vspace{-5pt}
\label{fig:add3}
\end{figure*}

%\clearpage
